# Supplementary material for: Rigorous construction of coherent state path integrals through dualization
Source: arXiv:1807.10462 source file (2018-07-27)
Supplement: Supplementary file 1 [file suppl.pdf]

# Rigorous construction of coherent state path integrals through dualization Supplemental material

Falk Bruckmann and Juan Diego Urbina

## ACTION (I) FAILS FOR THE HARMONIC OSCILLATOR

In the path integral weight with action (I), see Fig. 1, one uses the original symplectic term $z_k^*(z_k - z_{k+1})$, but shifts the second argument in the $H$-symbol to the time-slice of the first argument, $H(z_k^*, z_{k+1}) \to H(z_k^*, z_k)$ (assuming corrections to be suppressed in $\Delta$). Below Eq. (10) we show – using dual variables – that this action misses the ground states of $\hat{H}_q$. Here we demonstrate the same result for the harmonic oscillator, i.e. $\hat{H}_{q=1}$, by virtue of Gaussian integrals.

The path integral weight is

$$\int dz \, \exp\big( - \sum_{k,k'=1}^{N} z_k^* \, M^{k,k'} z_{k'} \big) = \frac{1}{\det M} \tag{i}$$

where in our case

$$M^{k,k'} = \delta_{k,k'} - \delta_{k,k'+1} + \Delta g \, \delta_{k,k'} \tag{ii}$$

with $N$-periodic boundary conditions, i.e. $M^{N,N+1} = -1$, too. The determinant of such a two-band matrix reads

$$\det M = \prod_{k=1}^{N}(1+\Delta g) - \prod_{k=1}^{N} 1 \to e^{\beta g} - 1$$
$$\frac{1}{\det M} \to \frac{1}{e^{\beta g}-1} = \sum_{n=1}^{\infty} e^{-\beta g n} \tag{iii}$$

which indeed misses the ground state at $n = 0$.

On the contrary, the correct description has an off-diagonal dynamical part $M_{q=1}^{k,k'} = \delta_{k,k'} - \delta_{k,k'+1} + \Delta g \, \delta_{k,k'+1}$, which translates into $\det M_{q=1} = \prod 1 - \prod(1-\Delta g) \to 1 - e^{-\beta g}$ and $1/\det M_{q=1} = 1/(1-e^{-\beta g}) = \sum_{n=0}^{\infty} e^{-\beta g n}$, which is the correct partition function (6).

## RE-ORDERING FORMULAS

### Normal ordering to particle number

One can easily check that normal ordered expressions of bosonic creation and annihilation operators can be expressed in terms of the number operator $\hat{n} = \hat{b}^\dagger \hat{b}$ as

$$(\hat{b}^\dagger)^q (\hat{b})^q = \hat{n}(\hat{n}-1)\dots(\hat{n}-q+1) \tag{iv}$$
$$= (\hat{n})_q = \sum_{r=0}^{q} S_1 \binom{q}{r} \hat{n}^r \tag{v}$$

as used in the body of the paper, between Eqs. (5) and (6). The second line refers to the falling factorial and its representation with (signed) Stirling numbers of the first kind $S_1\binom{\cdot\cdot}{\cdot\cdot}$.

### Particle number to anti-normal ordering

Powers of the particle number operator can be anti-normal ordered as follows:

$$\hat{n}^q = \sum_{r=0}^{q} (-1)^{q+r} S_2 \binom{q+1}{r+1} (\hat{b})^r (\hat{b}^\dagger)^r \tag{vi}$$

where $S_2\binom{\cdot\cdot}{\cdot\cdot}$ are the Stirling numbers of second kind. As an application consider powers of the third spin operator in the Schwinger boson representation $\hat{S}_z^q \sim (\hat{n}_1 - \hat{n}_2)^q$ as below Eq. (20). Since $\hat{n}_1$ and $\hat{n}_2$ commute, one needs to anti-order powers like in Eq. (vi) above to calculate $h$-symbols,

$$h_{\hat{n}^q}(z^*, z) = \sum_{r=0}^{q} (-1)^{q+r} S_2 \binom{q+1}{r+1} \rho^r \tag{vii}$$

where $\rho^2 = |z|$ and the $\mathcal{H}$-symbol via a Laguerre transform,

$$\mathcal{H}_{\hat{n}^q}(m) = \sum_{r=0}^{q} (-1)^{q+r} S_2 \binom{q+1}{r+1} \frac{(m+r)!}{m!} = m^q \tag{viii}$$

which proves the statement below Eq. (10) about the identical functional form of $\mathcal{H}(m)$ and $\hat{H}(\hat{n})$, when the latter depends on the particle number operator only.

### Normal to anti-normal ordering

For computing the $h$-symbol and $\mathcal{H}$-symbol (Eq. (10)) of $\hat{H}_q$, one needs to combine the two formulas above,

$$(\hat{b}^\dagger)^q (\hat{b})^q = \sum_{s=0}^{q} \sum_{r=0}^{s} (-1)^{s+r} S_1 \binom{q}{s} S_2 \binom{s+1}{r+1} (\hat{b})^r (\hat{b}^\dagger)^r$$
$$= \sum_{r=0}^{q} (-1)^{r+q} \frac{(q!)^2}{(r!)^2 (q-r)!} (\hat{b})^r (\hat{b}^\dagger)^r \tag{ix}$$

as used below Eq. (6), and obtains,

$$h_q(z^*, z) = (-1)^q q! \sum_{r=0}^{q} \binom{q}{r} \frac{(-1)^r}{r!} \rho^r = (-1)^q q!\, L_q(\rho) \tag{x}$$

$$\mathcal{H}_q(m) = (-1)^q q! \sum_{r=0}^{q} \binom{q}{r} \frac{(-1)^r}{r!} \frac{(m+r)!}{m!} = \frac{m!}{(m-q)!} \tag{xi}$$

## DUAL TREATMENT OF THE $H$-SYMBOL

Here we demonstrate how the dual variable treatment works with the symbol $H$, which is not diagonal in time slices and generically complex. Let us focus first on the Hamiltonian (5) with one fixed power $q$. In the analogue of Eq. (8), the weights $1 - \Delta H$ with the corresponding symbol $H(z_k^*, z_{k+1}) = g(\rho_k \rho_{k+1})^{q/2} e^{-i(\varphi_k - \varphi_{k+1})q}$ are naturally labeled with new dual variables $l_k$ being 0 or 1:

$$1 - \Delta H(z_k^*, z_{k+1}) = \sum_{l_k=0}^{1} (-\Delta g)^{l_k} \times (\rho_k \rho_{k+1})^{q l_k/2}\, \mathrm{e}^{-i(\varphi_k - \varphi_{k+1}) q l_k} \tag{xii}$$

for $k = 1, \dots N$ and with boundary conditions $(\rho, \varphi)_{N+1} = (\rho, \varphi)_1$. The partition function becomes

$$\mathcal{Z}_{H_q}^{(N)} = \prod_{k=1}^{N} \sum_{m_k=0}^{\infty} \sum_{l_k=0}^{1} \int_0^{2\pi} \frac{d\varphi_k}{2\pi}\, \mathrm{e}^{-i\varphi_k (n_k - n_{k-1})} \times \frac{(-\Delta g)^{l_k}}{m_k!} \int_0^{\infty} d\rho_k\, \mathrm{e}^{-\rho_k}\, \rho_k^{(n_k + n_{k-1})/2} \tag{xiii}$$

where $(l, m, n)_0 = (l, m, n)_N$ and where we have defined the following combination

$$n_k = (m + q\, l)_k \tag{xiv}$$

that (and not just $m_k$ as in the case of the $h$-symbol) is obviously kept constant, $n_k = n$, by the $\varphi_k$-integrations,

$$\mathcal{Z}_{H_q}^{(N)} = \sum_{n=0}^{\infty} \prod_{k=1}^{N} \sum_{l_k=0}^{1} \frac{(-\Delta g)^{l_k}}{(n - q l_k)!} \int_0^{\infty} d\rho_k\, \mathrm{e}^{-\rho_k}\, \rho_k^{n} \tag{xv}$$

The demand that $m_k = n - q\, l_k \geq 0$ has been taken care of by the factorial in the denominator. The $l_k$-sums can be written out to get

$$\mathcal{Z}_{H_q}^{(N)} = \sum_{n=0}^{\infty} \prod_{k=1}^{N} [1 - \frac{\Delta g}{(n-q)!}\, n!] \to \sum_{n=0}^{\infty} e^{-\beta g \frac{n!}{(n-q)!}} \tag{xvi}$$

which is the correct result, Eq. (6).

Due to linearity in the symbols this treatment is also possible for more than one power $q$, i.e. for $\hat{H} = \sum_q g_q (\hat{b}^\dagger)^q (\hat{b})^q$: one has to expand the $H$-symbol with several dual variables $l_k^{(q)}$. In analogy to Eq. (xiv) their sum $(m + \sum_q q\, l^{(q)})_k = n$ is constant and again appears as the power of $\rho_k$'s turning the $\rho_k$-integrals into $n!$. Since in the square bracket of Eq. (xvi), terms of order $\Delta^{0,1}$ are collected, one now gets a sum over all terms, where at most one $l^{(q)}$ is unity, i.e. $[1 - \Delta \sum_q \frac{g_q}{(n-q)!}\, n!]$, which exponentiates to the correct result.
